# Supplementary material for: Gaussian Processes for Demand Unconstraining
Source: arXiv:1711.10910 ancillary file (2017-11-29)
Supplement: Supplementary file 1 [file GP_Demand_Unconstraining_Supp_Mat_I_Price_J_Fowkes_D_Hopman.pdf]

Gaussian Processes for Demand Unconstraining — Supplementary Material

Ilan Price[a,*], Jaroslav Fowkes[a,], Daniel Hopman[a,b,]

[a] *Oxford-Emirates Data Science Lab, Mathematical Institute, University of Oxford, UK.*
[b] *Vrije Universiteit, Amsterdam, Netherlands*

# Additional Notation

Let $I_D$ be the index set of $\mathcal{D}$, such that $\mathcal{D} = \{d_i : i \in I_D\}$, where each $d_i$ is an observed demand value. Similarly we define $I_T$, $I_C$, and $I_U$ as the index sets of $\mathcal{D}_T$, $\mathcal{D}_C$, and $\mathcal{D}_U$, the true, constrained and unconstrained demand respectively, such that $\mathcal{D}_T = \{d_i : i \in I_T\}$, $\mathcal{D}_C = \{d_i : i \in I_C\}$, $\mathcal{D}_U = \{\hat{d}_i : i \in I_U\}$. Note that the index sets for constrained and unconstrained demand are the same, that is, $I_C = I_U$, since the elements $\hat{d}_i \in \mathcal{D}_U$ correspond to the unconstrained approximations of the elements $d_i \in \mathcal{D}_C$, and therefore $I_D = I_T \cup I_C = I_T \cup I_U$.

# Existing Unconstraining Methods

### Expectation Maximisation

The Expectation Maximisation (EM) algorithm is a well-established iterative algorithm for converging upon (local) maximum-likelihood estimates (MLE) of parameters for a given statistical model in the presence of some unobserved data. Stated in general terms, the algorithm works as follows: let $\mathcal{S}_1$ be a set of data points, let $\mathcal{S}_2$ be a set of latent or unobserved values, and let $\theta$ be a set of model parameters. The likelihood of the parameters is the probability of the data given those parameters, and thus the log-likelihood is given by

$$\log L(\theta; \mathcal{S}_1, \mathcal{S}_2) = \log p(\mathcal{S}_1, \mathcal{S}_2 | \theta). \tag{1}$$

The EM algorithm [4] applies two steps iteratively:

1. **E-step:** Calculate a new function $Q(\theta|\theta^{(t-1)})$, as the conditional expectation of the log-likelihood function in (1), given the conditional distribution of the unobserved variables $\mathcal{S}_2$ with the current parameter estimates $\theta^{(t-1)}$.
2. **M-step:** Maximise $Q(\theta|\theta^{(t-1)})$ with respect to $\theta$ to create new parameter estimates $\theta^{(t)}$.

*Corresponding author

*Email addresses:* ilan.price@maths.ox.ac.uk (Ilan Price), jaroslav.fowkes@maths.ox.ac.uk (Jaroslav Fowkes), daniel.hopman@maths.ox.ac.uk (Daniel Hopman)

EM is an unordered method, and uses the true observed demand values from a set of past flights (which are assumed to have a similar underlying demand pattern) to unconstrain demand for a set of constrained flights. For example, consider the set of $n+m$ demand curves corresponding to $n+m$ different flights, $m$ of which were constrained for a period of time, and $n$ of which were not. Let us assume we want to unconstrain the final cumulative demand totals before departure, as is commonly the case. EM takes the observations of true demand $\mathcal{D}_T$ as the final cumulative demand totals of the curves which were not constrained, and the observations of constrained demand $\mathcal{D}_C$ to be the observed cumulative totals of the booking curves which were each constrained by some imposed booking limit in $\mathcal{B} = \{b_i : i \in I_C\}$, such that $d_i = b_i$ for all $i \in I_C$.

EM assumes that the data is produced by the following statistical model: (i) the underlying demand distribution is normal, with some mean $\mu$ and standard deviation $\sigma$, which in 1D has the form

$$\phi(x;\mu,\sigma) = \frac{1}{\sqrt{2\pi}\sigma} \exp\left(\frac{-(x-\mu)^2}{2\sigma^2}\right); \tag{2}$$

(ii) all observations are sampled independently from this same distribution; and (iii) the constrained observations appear randomly in the sample. Given this statistical model, our log-likelihood function from Equation (1) becomes

$$\log L(\mu,\sigma;\mathcal{D}) = -\frac{n+m}{2}\log 2\pi - (n+m)\log\sigma - \frac{\sum_{i\in I_D}(d_i-\mu)^2}{2\sigma^2}. \tag{3}$$

*Applying the EM Algorithm*

*Initialisation*

To initialise the EM algorithm, we need to choose starting values $\mu^{(0)}$ and $\sigma^{(0)}$. The standard choice in the literature is to initialise these as the mean and standard deviation of all true demand observations ($\mathcal{D}_T$) [5, 6]. We must also define a convergence criterion, which requires choosing a small positive number $\varepsilon$ such that the algorithm will terminate once $|\mu^{(k)} - \mu^{(k-1)}| < \varepsilon$ and $|\sigma^{(k)} - \sigma^{(k-1)}| < \varepsilon$.

*Until convergence, do:*

*E-Step:* Calculate

$$Q(\mu,\sigma|\mu^{(k-1)},\sigma^{(k-1)}) = \mathbb{E}_{\mathcal{D}_C|\mathcal{D}_T,\mu^{(k-1)},\sigma^{(k-1)}}[\log L(\mu,\sigma;\mathcal{D})]. \tag{4}$$

Given the linearity of expectation, this expression is equivalent to

$$Q(\mu,\sigma|\mu^{(k-1)},\sigma^{(k-1)}) = \\ -\frac{n+m}{2}\log 2\pi - (n+m)\log\sigma - \frac{\sum_{i\in I_T}(d_i-\mu)^2}{2\sigma^2} - \frac{\sum_{i\in I_C}\mathbb{E}[d_i^2] - 2\mathbb{E}[d_i]\mu + \mu^2}{2\sigma^2},$$

where the expectation in the last term denotes the conditional expectation which is written in full in Equation (4).

In other words, the E-step involves calculating the expectation of all constrained values $\mathbb{E}[d_i]$, as well as $\mathbb{E}[d_i^2]$, for all $i \in I_C$, conditional on the fact that (i) $d_i$ come from a normal distribution with mean $\mu^{(k-1)}$

and standard deviation $\sigma^{(k-1)}$, and (ii) that $d_i$ must be greater than or equal to its constrained value (since the unconstrained value must of course be greater than or equal to the constrained value). Therefore, we calculate the expectations

$$\hat{d_i}^{(k-1)} = \mathbb{E}[d_i | d_i \geq b_i, d_i \sim \mathcal{N}(\mu^{(k-1)}, (\sigma^{(k-1)})^2)], \tag{5}$$

and

$$(\hat{d_i^2})^{(k-1)} = \mathbb{E}[d_i^2 | d_i \geq b_i, d_i \sim \mathcal{N}(\mu^{(k-1)}, (\sigma^{(k-1)})^2)]. \tag{6}$$

To calculate $\mathbb{E}[d^2 | d \geq b, d \sim \mathcal{N}(\mu, \sigma^2)]$ (having dropped the subscript $i$ and superscript $(k-1)$ for notational clarity)[1], we begin by noting that the distribution of $d \sim \mathcal{N}(\mu, \sigma^2)$ is the same as the distribution of $\sigma Z + \mu$, where $Z \sim \mathcal{N}(0, 1)$. Let $\phi(z)$ and $\Phi(z)$ denote the probability density function and cumulative distribution function of the standard normal distribution, respectively, and define $t = (b - \mu)/\sigma$. Then

$$\begin{aligned} \mathbb{E}[d^2 | d \geq b, d \sim \mathcal{N}(\mu, \sigma^2)] &= \mathbb{E}[(\sigma Z + \mu)^2 | Z \geq t, Z \sim \mathcal{N}(0, 1)] &(7)\\ &= \sigma^2 \mathbb{E}[Z^2 | Z \geq t] + 2\mu\sigma \mathbb{E}[Z | Z \geq t] + \mu^2 \mathbb{E}[1 | Z \geq t], &(8) \end{aligned}$$

and each term in this expression can be evaluated independently. Consider the first term,

$$\mathbb{E}[Z^2 | Z \geq t] = \frac{\int_t^\infty z^2 \phi(z) \mathrm{d}z}{p(Z \geq t)}. \tag{9}$$

The standard normal distribution has the property that $\phi'(z) = -z\phi(z)$, and $S(t) = 1 - \Phi(t) = \int_t^\infty \phi(z) \mathrm{d}z = p(Z \geq t)$ is referred to as the survival function. Substituting these into Equation (9) gives

$$\mathbb{E}[Z^2 | Z \geq t] = -\frac{\int_t^\infty z\phi'(z) \mathrm{d}z}{S(t)}. \tag{10}$$

Using integration by parts and the fundamental theorem of calculus, we derive that

$$\mathbb{E}[Z^2 | Z \geq t] = \frac{t\phi(t)}{S(t)} + 1. \tag{11}$$

Similarly (though without the need to integrate by parts), it can be shown that

$$\mathbb{E}[Z | Z \geq t] = \frac{\phi(t)}{S(t)}, \quad \text{and} \quad \mathbb{E}[1 | Z \geq t] = 1. \tag{12}$$

Putting these all together we have that

$$\mathbb{E}[d^2 | d \geq b, d \sim \mathcal{N}(\mu, \sigma^2)] = \sigma^2 \left( \frac{t\phi(t)}{S(t)} + 1 \right) + 2\mu\sigma \left( \frac{\phi(t)}{S(t)} \right) + \mu^2, \tag{13}$$

where $t = (b - \mu)/\sigma$.

We note here the importance of calculating the conditional expectations $\mathbb{E}[d_i]$ and $\mathbb{E}[d_i^2]$ separately. It appears that a number of sources make the mistake of simply calculating $\hat{d_i}^{(k-1)} = \mathbb{E}[d_i]$ for all $i \in I_C$, and

[1] We omit the details for calculating the expression in Equation (5) since these should be clear from this explanation of how to calculate the expression in Equation (6).

substituting these into the log-likelihood function given in Equation (3) in place of the constrained values $d_i$. This is in fact a significant statistical error, since doing so implicitly makes the assumption that $\mathbb{E}[d_i^2] = \mathbb{E}[d_i]^2$, which of course is false.[2]

*M-Step:* Next, we maximise our function $Q$ with respect to $\mu$ and $\sigma$ to calculate $\mu^{(k)}$ and $\sigma^{(k)}$, which are given by the expressions,

$$\mu^{(k)} = \frac{1}{m+n}\left(\sum_{i \in I_T} d_i + \sum_{i \in I_C} \hat{d}_i^{(k-1)}\right), \tag{14}$$

$$\sigma^{(k)} = \frac{1}{\sqrt{m+n}}\left(\sum_{i \in I_T} (d_i - \mu)^2 + \sum_{i \in I_C}\left((\hat{d_i^2})^{(k-1)} - 2\hat{d}_i^{(k-1)}\mu + \mu^2\right)\right)^{\frac{1}{2}}, \tag{15}$$

where $\hat{d}_i^{(k-1)}$ and $(\hat{d_i^2})^{(k-1)}$ are the conditional expectations calculated in the E-Step.

Once the algorithm has converged after, say, $K$ iterations, the estimates $\mu^{(K)}$ and $\sigma^{(K)}$ can be used to unconstrain the constrained demand observations, by calculating $\mathbb{E}[d_i | d_i \geq b_i, X \sim \mathcal{N}(\mu^{(K)}, (\sigma^{(K)})^2)]$, for all $i \in I_C$.

**Projection Detruncation**

Projection Detruncation (PD) is a variant of EM proposed by Hopperstad in 1995 [2]. The key difference between EM and PD is that where EM calculates $\hat{d}_i^{(k-1)}$ to be the mean of the conditional distribution, PD instead calculates $\hat{d}_i^{(k-1)}$ to be a pre-specified percentile on the conditional distribution, such that $\hat{d}_i^{(k-1)}$ satisfies

$$p(d_i > \hat{d}_i^{(k-1)} | d_i > b_i, \mu^{(k-1)}, \sigma^{(k-1)}) = \tau, \tag{16}$$

for some pre-specified value of $\tau$.[3] For example, when $\tau = 0.5$ we can see that $\hat{d}_i^{(k-1)}$ corresponds to the median of the conditional distribution. To calculate $\hat{d}_i^{(k-1)}$ we note that Equation (16) can be written equivalently as

$$p(d_i > \hat{d}_i | \mu^{(k-1)}, \sigma^{(k-1)}) = \tau p(d_i > b_i | \mu^{(k-1)}, \sigma^{(k-1)}), \tag{17}$$

and therefore as

$$\int_{\hat{d}_i^{(k-1)}}^{\infty} \phi(x | \mu^{(k-1)}, \sigma^{(k-1)}) \mathrm{d}x = \tau \int_{b_i}^{\infty} \phi(x | \mu^{(k-1)}, \sigma^{(k-1)}) \mathrm{d}x, \tag{18}$$

which is the equation solved at each iteration for every $\hat{d}_i^{(k-1)}$ [6]. PD then constructs a function $\hat{Q}(\mu, \sigma)$ by taking the log-likelihood function in Equation (3) and replacing each constrained observation $\{d_i : i \in I_C\}$

[2]If this were true, the variance $\mathrm{var}[X] = \mathbb{E}[X^2] - \mathbb{E}[X]^2$ would always be zero.

[3]Throughout our paper, when we apply PD we do so with $\tau = 0.5$.

with $\hat{d}_i^{(k-1)}$.[4] Substituting these values into the log-likelihood function yields

$$\hat{Q}(\mu,\sigma) = -\frac{m+n}{2}\log 2\pi - (m+n)\log\sigma - \frac{\sum_{i\in I_T}(d_i-\mu)^2}{2\sigma^2} - \frac{\sum_{i\in I_C}(\hat{d}_i^{(k-1)}-\mu)^2}{2\sigma^2}. \tag{19}$$

$\hat{Q}(\mu,\sigma)$ is then maximised with respect to $\mu$ and $\sigma$ to calculate new parameter estimates just as in the M-step of EM, such that

$$\mu^{(k)} = \frac{1}{m+n}\left(\sum_{i\in I_T} d_i + \sum_{i\in I_C}\hat{d}_i^{(k-1)}\right), \tag{20}$$

$$\sigma^{(k)} = \frac{1}{\sqrt{m+n}}\left(\sum_{i\in I_T}(d_i-\mu)^2 + \sum_{i\in I_C}(\hat{d}_i^{(k-1)}-\mu)^2\right)^{\frac{1}{2}}. \tag{21}$$

Once (if) the algorithm converges,[5] after, say, $K$ iterations, then the estimates $\mu^{(K)}$ and $\sigma^{(K)}$ can be used to calculate the unconstrained demand values in $\mathcal{D}_U$ by solving

$$\int_{\hat{d}_i}^{\infty} f(x|\mu^{(K)},\sigma^{(K)})\mathrm{d}x = \tau\int_{b_i}^{\infty} f(x|\mu^{(K)},\sigma^{(K)})\mathrm{d}x, \tag{22}$$

for $\hat{d}_i$, for all $i \in I_C$ [6].

### Double Exponential Smoothing

Double Exponential Smoothing (DES) is a smoothing method commonly used for forecasting based on data which displays some trend behaviour (which is clearly present in most bookings data). Queenan et al. [5] therefore propose using "Holt's method" (one variant of DES) for the purposes of unconstraining demand.

DES is a time-series method and is applied to one constrained curve at a time, as follows [5]: let $t_0$ be the day the fare-class is made available for booking, let $t_B$ be the day on which bookings become constrained ($t_0 < t_B$), and let $A_i$ be the actual cumulative demand at time $t_i$. We define $F_i$ and $M_i$ as the smoothed base and trend components for time period $t_i$, respectively, and two smoothing constants $\alpha$ and $\beta$ ($0 < \alpha, \beta < 1$). We then initialise the base and trend components at $t_0$ as

$$F_0 = A_0, \tag{23}$$

$$M_0 = (A_B - A_0)/B, \tag{24}$$

and proceed forward in time by calculating

$$F_i = \alpha A_i + (1-\alpha)(F_{i-1} + M_{i-1}), \tag{25}$$

$$M_i = \beta(F_i - F_{i-1}) + (1-\beta)M_{i-1}, \tag{26}$$

for $i \in \{1,\ldots,B\}$. The method works by smoothing the base and trend components separately at each time period $t_i$. The new base component $F_i$ is a weighted average of two terms: the first is the actual demand at

[4]Note that for PD there is no need to calculate $\hat{d}_i$ and $(\hat{d}_i)^2$ separately.

[5]Unlike for EM, there is no formal convergence result for PD.

time $t_i$; the second can be thought of as a forecasted demand for time $t_i$, calculated by adding the previous base and trend components. The new trend component $M_i$ is calculated as a weighted average of the previous trend component, and the change in the smoothed base component between time $t_{i-1}$ and time $t_i$.

The values of the smoothing parameters $\alpha$ and $\beta$ are chosen by minimising the sum of the squares of the forecast errors for $i \in \{1, \ldots, B\}$,

$$\min_{\alpha,\beta} \sum_{i=1}^{B} (A_i - F_{i-1} - M_{i-1})^2. \tag{27}$$

Though this problem is non-convex in $\alpha$ and $\beta$, the range of possible values is small enough that a brute force optimisation routine (i.e. evaluating the objective function on a grid of points) is efficient enough for practical purposes.

To forecast the unconstrained cumulative demand $d$ for, say, 20 time periods beyond $t_B$, we simply calculate

$$d_{B+20} = F_B + 20M_B. \tag{28}$$

# Proof of Positive Semi-Definiteness

Recall the variable-degree polynomial kernel from Section 4 of the accompanying paper, which results in a covariance matrix of the form

$$\mathbf{K} = \sigma^2(\mathbf{x}\mathbf{x}^\top + c\mathbf{e}\mathbf{e}^\top)^{\diamond p}.$$

Here we show that the matrix $A = \mathbf{x}\mathbf{x}^\top + c\mathbf{e}\mathbf{e}^\top$ is PSD so long as $c > 0$ and every element of $\mathbf{x}$ is non-negative, where $\mathbf{x}, \mathbf{e} \in \mathbb{R}^n$ and $\mathbf{e}$ is the vector of all ones.

Giraudo [1] shows how to find the eigenvalues of a rank-two matrix. We know that there are at most two distinct non-zero eigenvalues $\lambda_1$ and $\lambda_2$. We have that

$$\mathrm{Tr}(A) = ||\mathbf{x}||_2^2 + c||\mathbf{e}||_2^2 = \lambda_1 + \lambda_2, \tag{29}$$

and

$$\begin{aligned}
\mathrm{Tr}(A^2) &= \mathrm{Tr}(\mathbf{x}\mathbf{x}^\top\mathbf{x}\mathbf{x}^\top + 2c\mathbf{e}\mathbf{e}^\top\mathbf{x}\mathbf{x}^\top + c^2\mathbf{e}\mathbf{e}^\top\mathbf{e}\mathbf{e}^\top), && (30)\\
&= ||\mathbf{x}||_2^4 + c^2||\mathbf{e}||_2^4 + 2c\langle\mathbf{x},\mathbf{e}\rangle^2, && (31)\\
&= (\lambda_1 + \lambda_2)^2 - 2c||\mathbf{x}||_2^2||\mathbf{e}||_2^2 + 2c\langle\mathbf{x},\mathbf{e}\rangle^2. && (32)
\end{aligned}$$

Since

$$2\lambda_1\lambda_2 = (\lambda_1 + \lambda_2)^2 - \lambda_1^2 - \lambda_2^2, \tag{33}$$

we have that

$$\lambda_1\lambda_2 = c||\mathbf{x}||_2^2||\mathbf{e}||_2^2 - c\langle\mathbf{x},\mathbf{e}\rangle^2. \tag{34}$$

This allows us to write an equation for the non-zero eigenvalues

$$\lambda^2 - (||\mathbf{x}||_2^2 + c||\mathbf{e}||_2^2)\lambda + c||\mathbf{x}||_2^2||\mathbf{e}||_2^2 - c\langle\mathbf{x},\mathbf{e}\rangle^2 = 0. \tag{35}$$

The discriminant is given by

$$\Delta = (||\mathbf{x}||_2^2 + c||\mathbf{e}||_2^2)^2 - 4(c||\mathbf{x}||_2^2||\mathbf{e}||_2^2 - c\langle\mathbf{x},\mathbf{e}\rangle^2) = (||\mathbf{x}||_2^2 - c||\mathbf{e}||_2^2)^2 + 4c\langle\mathbf{x},\mathbf{e}\rangle^2 > 0, \tag{36}$$

and the non-zero eigenvalues are given by

$$\lambda_\pm = \frac{||\mathbf{x}||_2^2 + c||\mathbf{e}||_2^2 \pm \sqrt{(||\mathbf{x}||_2^2 - c||\mathbf{e}||_2^2)^2 + 4c\langle\mathbf{x},\mathbf{e}\rangle^2}}{2}. \tag{37}$$

Thus to show that the matrix is PSD we need to show that

$$||\mathbf{x}||_2^2 + c||\mathbf{e}||_2^2 \geq \sqrt{(||\mathbf{x}||_2^2 - c||\mathbf{e}||_2^2)^2 + 4c\langle\mathbf{x},\mathbf{e}\rangle^2}. \tag{38}$$

Now, as $\mathbf{e}$ is the vector of ones and $x_i \geq 0$ for $i = 1,\ldots,n$, we have that

$$c||\mathbf{e}||_2^2 = c\langle\mathbf{e},\mathbf{e}\rangle = nc, \tag{39}$$

and

$$\langle\mathbf{x},\mathbf{e}\rangle = x_1 + x_2 + \cdots + x_n = ||\mathbf{x}||_1. \tag{40}$$

We prove the inequality in (38) by contradiction. Assume

$$||\mathbf{x}||_2^2 + c||\mathbf{e}||_2^2 < \sqrt{(||\mathbf{x}||_2^2 - c||\mathbf{e}||_2^2)^2 + 4c\langle\mathbf{x},\mathbf{e}\rangle^2}. \tag{41}$$

Then

$$\begin{aligned}
 & ||\mathbf{x}||_2^2 + nc & < \sqrt{(||\mathbf{x}||_2^2 - nc)^2 + 4c||\mathbf{x}||_1^2}, \quad (42)\\
\iff \quad & ||\mathbf{x}||_2^4 + 2nc||\mathbf{x}||_2^2 + n^2c^2 & < ||\mathbf{x}||_2^4 - 2nc||\mathbf{x}||_2^2 + n^2c^2 + 4c||\mathbf{x}||_1^2, \quad (43)\\
\iff \quad & n||\mathbf{x}||_2^2 & < ||\mathbf{x}||_1^2, \quad (44)\\
\iff \quad & \sqrt{n}||\mathbf{x}||_2 & < ||\mathbf{x}||_1. \quad (45)
\end{aligned}$$

However, using Cauchy-Schwarz we have that

$$||\mathbf{x}||_1 = \sum_{i=1}^n |x_i| = \sum_{i=1}^n |x_i| \cdot 1 \leq \left(\sum_{i=1}^n |x_i|^2\right)^{1/2} \left(\sum_{i=1}^n 1^2\right)^{1/2} = \sqrt{n}||\mathbf{x}||_2, \tag{46}$$

which contradicts the result in (45). □

# Numerical Experiments

### Creation of Booking Limits in Experiment 1

To generate the booking limits for each of the 100 curves, Queenan et al. use the fact that the set of total demand is approximately normally distributed. First, they calculate the mean $\mu$ and standard deviation $\sigma$ of this set of total demand. They then use the $z$-scores from a standard normal distribution which correspond to 20, 40, 60, 80, and 98% of data being above that level; that is, $z_{20}$ is the number of standard deviations away from zero such that 20% percentage of the area under the normal distribution is to the right of this point, and so on for $z_{40}$, $z_{60}$, $z_{80}$, and $z_{98}$. These $z$-scores are then used to create new 'mean booking limits' for each proportion of constrained curves, according to $\mu_{20} = \mu + z_{20}\sigma$, and so on. To create the booking limits for the 20% constrained case, they randomly sample 100 booking limits from a normal distribution with mean $\mu_{20}$ and standard deviation $\sigma$, one for each booking curve. If the booking limit is lower than the total demand of the corresponding curve, then that curve is constrained by its booking limit. This same procedure is followed to create the booking limits to constrain 40, 60, 80, and 98% of the curves.

### E3 Error Table for Experiment 1

| | Proportion of Days Constrained | | | | |
|---|---|---|---|---|---|
| Prop. Constrained | 20% | 40% | 60% | 80% | 98% |
| | | | Convex | | |
| EM | 12.74 | 15.10 | 15.87 | 17.21 | 22.31 |
| PD | 13.26 | 16.01 | 16.61 | 19.27 | 26.26 |
| DES | 4.51 | 4.82 | 5.70 | 6.13 | 8.17 |
| **EM Daily** | **3.98** | **4.11** | **4.73** | **5.25** | **6.49** |
| PD Daily | 4.01 | 4.12 | 4.74 | 5.27 | 6.56 |
| GPs | 4.37 | 5.24 | 5.74 | 6.08 | 8.11 |
| | | | Concave | | |
| EM | 12.45 | 15.64 | 16.51 | 18.56 | 22.20 |
| PD | 12.88 | 15.67 | 17.34 | 21.40 | 29.61 |
| DES | 11.43 | 12.95 | 17.65 | 21.93 | 34.68 |
| EM Daily | 3.90 | 4.20 | 4.59 | 5.36 | 6.91 |
| **PD Daily** | **3.59** | **4.02** | **4.46** | **5.10** | **6.33** |
| GPs | 6.11 | 7.40 | 8.05 | 11.24 | 15.14 |
| | | | Homogeneous | | |
| EM | 14.37 | 15.07 | 15.34 | 17.31 | 23.04 |
| PD | 14.22 | 14.76 | 16.82 | 20.13 | 27.25 |
| DES | 4.45 | 5.18 | 5.81 | 6.23 | 7.93 |
| **EM Daily** | **3.79** | **3.98** | 5.33 | **5.58** | **6.83** |
| PD Daily | 3.84 | 4.01 | 5.35 | 5.61 | 7.05 |
| GPs | 3.93 | 4.28 | **5.26** | 5.70 | 7.69 |

Table 1: Average absolute error in final cumulative demand (E3) in Experiment 1. These results measure how close the unconstrained approximations of total demand were to the actual demand totals on average.

### Creation of Booking Curves in Experiment 2

The sets of curves used in Experiment 2 were created as follows: the number of bookings for each day before departure was generated by sampling from a Poisson distribution with the corresponding rate $\lambda$ for that day (e.g. bookings 100 days before departure are sampled from a Poisson distribution with mean $\lambda(-100)$, etc.). The specific functions $\lambda(t)$ used for each set of demand curves were:

*Concave*

$$\textbf{Linear} : \lambda(t) = \frac{-11}{140} t.$$
$$\textbf{Quadratic} : \lambda(t) = \frac{19}{28000} t^2.$$
$$\textbf{Cubic} : \lambda(t) = \frac{-1}{140000} t^3.$$

*Convex*

$$\textbf{Linear} : \lambda(t) = \frac{9.3}{140}(t + 140).$$
$$\textbf{Quadratic} : \lambda(t) = \frac{1}{1400}(t + 140)^2.$$
$$\textbf{Cubic} : \lambda(t) = \frac{1}{119000}(t + 140)^3.$$

In Figure 1 we show sample data created by each of the linear, quadratic and cubic rates in the convex case.

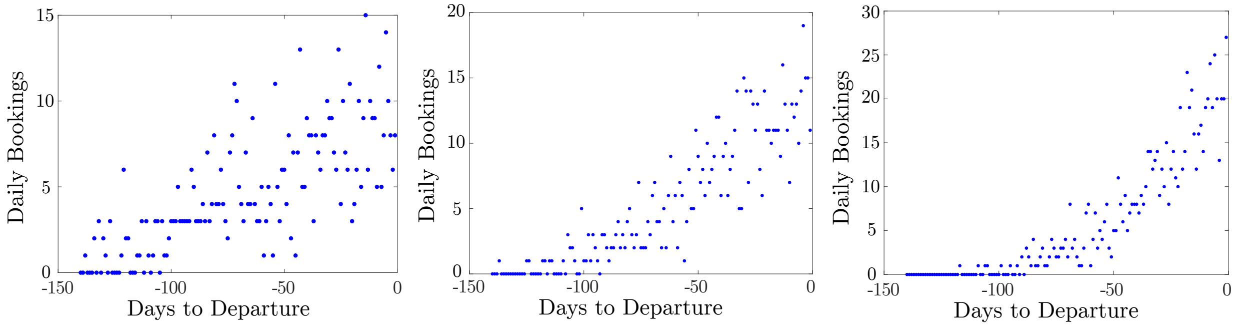


(a) Linear $\lambda(t)$ (b) Quadratic $\lambda(t)$ (c) Cubic $\lambda(t)$

Figure 1: Examples of data generated to create the set of convex curves used in Experiment 2. The data was generated by sampling bookings on day $t$ from a Poisson distribution with mean $\lambda(t)$. For 30 curves $\lambda(t)$ was linear, resulting in data resembling those in Figure (a), for 30 curves $\lambda(t)$ was quadratic, resulting in data resembling those in Figure (b), and for the final 30 curves $\lambda(t)$ was cubic resulting in data resembling those in Figure (c).

**Non-Homogeneous Poisson Process Simulation**

One standard algorithm for simulating a non-homogeneous Poisson process (NHPP) is known as 'thinning' [3], which works as follows: given a Poisson rate $\lambda(t)$, choose a $\bar{\lambda}$ such that $\lambda(t) \leq \bar{\lambda}$ for all $t$ in the period being considered. The following algorithm generates the arrival times $T_i \in [0, T_{final}]$, at which arrivals (bookings) are sampled from a Poisson distribution with mean $\lambda(T_i)$.

---

**Algorithm 1** Thinning Algorithm for Generating Arrival Times of a NHPP

---

Set $i = 0$, $T_0 = 0$, $T^* = 0$
**while** $T^* \leq T_{final}$ **do**
    $i = i + 1$
    (1) Generate an exponential random variable E with parameter $\bar{\lambda}$
    (2) Set $T^* = T^* + E$
    (3) Sample a number $u \in [0, 1]$ from a uniform distribution
    **if** $u > \lambda(T^*)/\bar{\lambda}$ **then**
        Reject the new $T^*$ and go back to Step (1)
    **else**
        Set $T_i = T^*$
    **end if**
**end while**

---

To represent this data in terms of daily bookings, we sum all arrivals made at different times on the same day and use the total as the single data point for that day.

In Figure 2 we plot our best attempt to generate data with this process which resembles real Emirates Airlines demand data. Though more realistic than the data from Experiments 1 and 2, this process does not reproduce real data as well as the DPP data used for Experiment 3.

**Creation of Booking Curves in Experiment 3**

The sets of curves used in Experiment 3 were created as per the process summarised in Figure 3. The lengths of the intervals between days on which bookings are made are sampled from a Poisson distribution with mean $\lambda_2(t)$, and the number of bookings for each day on which bookings are made is sampled from a Poisson distribution with rate $\lambda_1(t)$. The specific functions used for $\lambda_1(t)$ to create the data in Experiment 3 were

$$\textbf{Linear}: \lambda_1(t) = \frac{3}{140}(t + 140) + 1,$$
$$\textbf{Quadratic}: \lambda_1(t) = \frac{1}{7000}(t + 140)^2 + 1,$$
$$\textbf{Cubic}: \lambda_1(t) = \frac{1}{420000}(t + 140)^3 + 1,$$

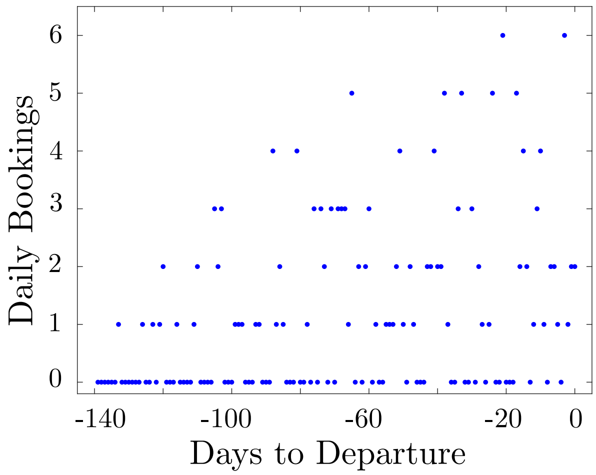


Figure 2: Daily bookings data produced by simulating a non-homogeneous Poisson process (NHPP). The NHPP was simulated using the thinning algorithm, with a linear $\lambda(t) = 0.0116(t+140)$, the specific formula for which was chosen so as to replicate on average a total cumulative demand similar to that of a typical high-demand curve from the Emirates data set discussed in Section 5.3 of the accompanying paper.

and the function $\lambda_2(t)$ was

$$\lambda(t) = \frac{1}{2100}t^2.$$

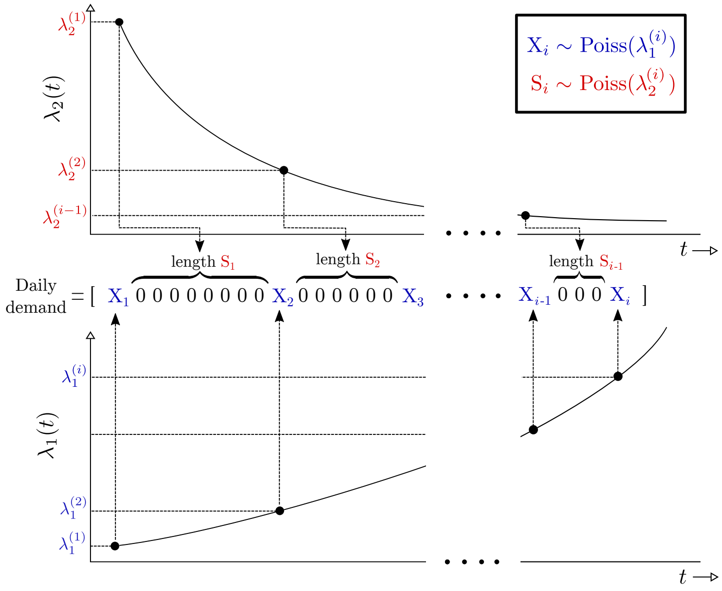


Figure 3: Schematic illustrating the procedure for producing 'DPP' test data in Experiment 3. The rate $\lambda_2(t)$ determines the days on which bookings are made by determining the number of days between bookings (denoted by $S_i$), while the rate $\lambda_1(t)$ determines how many bookings are made on those days (denoted by $X_i$).

# References


[1] Giraudo, D. (2012). Eigenvalues of a sum of rank-one matrices. Mathematics Stack Exchange. URL: `https://math.stackexchange.com/q/112201`.

[2] Hopperstad, C. (1995). An alternative detruncation method. *Boeing Commercial Aircraft Company Internal Document, Boeing, Renton, Wash, USA*, .

[3] Lewis, P. A., & Shedler, G. S. (1979). Simulation of nonhomogeneous Poisson processes by thinning. *Naval Research Logistics (NRL)*, *26*, 403–413.

[4] Moon, T. K. (1996). The expectation-maximization algorithm. *IEEE Signal Processing Magazine*, *13*, 47–60.

[5] Queenan, C. C., Ferguson, M., Higbie, J., & Kapoor, R. (2007). A Comparison of Unconstraining Methods to Improve Revenue Management Systems. *Production and Operations Management*, *16*, 729–746.

[6] Talluri, K. T., & Van Ryzin, G. J. (2006). *The theory and practice of revenue management*. Springer Science & Business Media.
